# Supplementary material for: Make the Pertinent Salient: Task-Relevant Reconstruction for Visual Control with Distractions
Source: arXiv:2410.09972 source file (2024-10-13)
Supplement: Supplementary file 1 [file Tab_Appendix_IoU.tex]

\begin{table}[h]
\caption{PerSAM's segmentation quality on train-time replay buffer measured by IoU.
}\label{tab:SAM_IoU}
\begin{adjustbox}{width=0.4\linewidth,center}
  \begin{tabular}{lc}
    \toprule
    Task & IoU \\
    \midrule
    Cartpole Swingup & 0.64 \\
    Cartpole Swingup Sparse & 0.62 \\
    Cheetah Run & 0.80 \\
    Hopper Stand & 0.48 \\
    Reacher Easy & 0.54 \\
    Walker Run & 0.76 \\
  \bottomrule
  \end{tabular}
  \end{adjustbox}
\end{table}
